# Supplementary material for: Encoded Value-at-Risk: A Predictive Machine for Financial Risk Management
Source: arXiv:2011.06742 source file (2020-11-13)
Supplement: Supplementary file 1 [file appendix.tex]

\section{Appendix: VAE Theory by Sina Seyfi}

There are a variety of methods to optimum loss function such as Gradient Descend. Therefor we can define the loss function as $$J(\theta) = |X - \hat{X}|^2$$
which measures difference between $X$ and $\hat{X}$ with MSE.

%%%%%%%%%%%%%%%%%%%%%%%%%%%%%%%%%%%%%%%%%%%%%%%%%%%%%%%%%%%%%%%%%%%%%%%

The KL divergence between $q_{\phi}(z)$ and $p(z)$ is supposed to be minimum in order to let $q_{\phi}(z)$ be a nice approximate of $p(z|x)$. The more similarity between $q_{\phi}(z)$ and $p(z|x)$, the less $\mathcal{KL}(q_{\phi}(z)||p(z|x))$. For calculating the integral in equation \ref{eq:2.3}, using Bayes' rule
\begin{equation}
    p(z|x) = \frac{p_{\theta}(x|z)p(z)}{p_{\theta}(x)} = \frac{p_{\theta}(x, z)}{p_{\theta}(x)}
\end{equation}

and substituting in \ref{eq:2.3}, we have: 

\begin{equation}
   \mathcal{KL}(q_{\phi}(z)||p(z|x)) = - \int  q_{\phi}(z) \log \frac{\frac{p_{\theta}(x,z)}{p_{\theta}(x)}}{q_{\phi}(z)} dz
    \end{equation}
\begin{equation}
       = - \int  q_{\phi}(z) \log[\frac{p_{\theta}(x,z)}{q_{\phi}(z)}.\frac{1}{p_{\theta}(x)}]dz
\end{equation}
\begin{equation}
    = - \int q_{\phi}(z)[\log \frac{p_{\theta}(x,z)}{q_{\phi}(z)} - \log p_{\theta}(x)] dz
\end{equation} 

\begin{equation} \label{eq:2.8}
    = - \int q_{\phi}(z)[\log p_{\theta}(x,z) - \log q_{\phi}(z)]dz + \int q_{\phi}(z) \log p_{\theta}(x) dz
\end{equation} 
Since the integral in second term is over $z$, and $\log p_{\theta}(x)$ is independent from $z$, so the equation \ref{eq:2.8} could rewrite as:
\begin{equation}
    \mathcal{KL}(q_{\phi}(z)||p(z|x)) = - \int q_{\phi}(z)[\log p_{\theta}(x,z) -\log p(z)]dz + \log p_{\theta}(x)\int q_{\phi}(z)  dz
\end{equation} 
It is obvious that $\int q(z)  dz = 1$. So, it becomes:

\begin{equation}
    \log p_{\theta}(x) = \mathcal{KL}(q_{\phi}(z)||p(z|x)) +  \int q_{\phi}(z)\log \frac{p_{\theta}(x,z)}{q_{\phi}(z)}dz
\end{equation}

Because the $x$ is input data and given, $\log p_{\theta}(x)$ is a constant aside from what $q_{\phi}$ is. Hence, to minimize the $\mathcal{KL}(q_{\phi}(z)||p(z|x))$, it is enough to maximize the $\int q_{\phi}(z)\log \frac{p_{\theta}(x,z)}{q_{\phi}(z)}dz$. Let say the $\mathcal{L}(\phi, \theta)$ is a variational lower bound to $p_{\theta}(x)$. So it can defined:

 \begin{equation} \label{eq:2.11}
    \mathcal{L}(\phi, \theta) = \int q_{\phi}(z)\log \frac{p_{\theta}(x,z)}{q_{\phi}(z)}dz
 \end{equation}
 
 the reason is the term $\mathcal{KL}(q_{\phi}(z)||p(z|x))  \geq  0$. Since, $\mathcal{L}{(\phi, \theta)}  \leq \log p_{\theta}(x)$, so $\mathcal{L}(\phi, \theta)$ could be a lower bound for $\log p_{\theta}(x)$. By substituting $p_{\theta}(x|z)p(z)$ instead of $p_{\theta}(x,z)$ It can write as equation \ref{eq:3}:

 \begin{equation} \label{eq:3}
  \mathcal{L}(\phi, \theta) = \int q_{\phi}(z)\log \frac{p_{\theta}(x|z)p(z)}{q_{\phi}(z)}dz
 \end{equation}
 
 \begin{equation} \label{eq:2.13}
  \mathcal{L}(\phi, \theta) =\int q_{\phi}(z)[\log p_{\theta}(x|z) + \log \frac{p(z)}{q_{\phi}(z)}]dz
 \end{equation}
 By segmenting the equation \ref{eq:2.13}, we have:
 \begin{equation} \label{eq:2.14}
     \mathcal{L}(\phi, \theta) = \int q_{\phi}(z) \log p_{\theta}(x|z) dz + \int q_{\phi}(z) \log \frac{p(z)}{q_{\phi}(z)} dz
 \end{equation}
 
The equation \ref{eq:2.14}, consists two parts. The term $\int q_{\phi}(z) \log p_{\theta}(x|z) dz$ shows the expectation of $\log p_{\theta}(x|z)$ with respect to $q_{\phi}(z)$ and the term $\int q_{\phi}(z) \log \frac{p(z)}{q_{\phi}(z)} dz$ represents the negative $\mathcal{KL}$ divergence between $q_{\phi}(z)$ and $p(z)$. So by substituting the $-\mathcal{KL}(q_{\phi}(z)||p(z))$ to this terms, the lower bound $\mathcal{L}(\phi, \theta)$ becomes:
\begin{equation} \label{eq:2.15}
    \mathcal{L}(\phi, \theta) = \mathbb{E}_{q_{\phi}(z)}[\log p_{\theta}(x|z)] - \mathcal{KL}(q_{\phi}(z)||p(z))
\end{equation}
 
The main goal is to maximize the lower bound $\mathcal{L}(\phi, \theta)$, because in this way, the $p_{\theta}(x)$ is going to be maximize either. according to equation \ref{eq:2.15} maximizing the $\mathcal{L}(\phi, \theta)$ is equivalent to minimize the $\mathcal{KL}(q_{\phi}(z)||p(z))$ and maximize the $\mathbb{E}_{q_{\phi}(z)}[\log p_{\theta}(x|z)]$, simultaneously. The first condition, leads to keep $q_{\phi}(z)$ similar to $p(z)$ and the second one, highs the likelihood of $x$ generated from $z$.
 
% \begin{center}
% \centering \includegraphics[scale=0.25]{Figures/p-q.jpg} 
% \end{center}

By assuming that the $q_{\phi}(z|x)$ and $p_{\theta}(x|z)$ are two neural network functions, which map input data $x$ to the latent layer $z$ and vice versa, the decoder will train to rebuild the $x$ from $z$ with respect to $\theta$. The neural network $q_{\phi}$ was defined because the distribution of input $x$ was not tractable. So $q_{\phi}$ must be in that way to be easily computable and also create $z$ in form of a normal distribution. In other words, we force the network to create latent layer $z$ in this way:
\begin{equation}
    p(z) = \mathcal{N}(\mu_{\phi}(x), \sigma_{\phi}(x) ^ 2  \times  I)
\end{equation}
Where $I$ is identity matrix. So $q_{\phi}$ must be able to map data $x$ (with any distribution) to a normal. necessarily, $p_{\theta}(\hat{x}|z)$ will learn to get some input with a normal distribution and maps them to the output of the decoder $\hat{x}$.

It should mentioned that the $q_{\phi}(z|x)$ can build the parameters of $z \sim \mathcal{N}(\mu_{\phi}(x), \sigma_{\phi}(x) ^ 2  \times  I)$ instead of building all of that. consequently, the latent layer $z$ has two terms: $\mu_{\phi}$ and $\sigma_{\phi}$. Then, it could sampled randomly from $z$ and pass it through the decoder, $p_{\theta}(\hat{x}|z)$, to generate new outputs, because $p_{\theta}(\hat{x}|z)$ has trained to make $\hat{x}$ from a normal distribution. Then, after training the encoder and decoder, simply we omit the encoder part and by sampling from $z$ and feed it to the decoder, we will give generated data which may not occurred beforehand necessarily, but they are probable. It stands to reason that the VAE is a generative model. 

The method we use for maximizing $\mathcal{L}(\phi, \theta)$ is stochastic gradient ascent. So we should compute $\nabla \mathcal{L}(\phi, \theta)$ with respect to $\phi$ and $\theta$. According to equation \ref{eq:2.11} we can say:
\begin{equation} \label{eq:2.17}
     \mathcal{L}(\phi, \theta) = \mathbb{E}_{q_{\phi}(z)}[\log \frac{p(z)p_{\theta}(x|z)}{q_{\phi}(z)}]
\end{equation}
For computing $\nabla_{\theta} \mathcal{L}(\phi, \theta)$ we will estimate $\mathcal{L}(\phi, \theta)$ using Monte Carlo estimate, by sampling $\{z_{i}\}_{i=1} ^ s$ from the latent space $z$, which $s$ is the number of samples:

\begin{equation}
    \mathcal{L}(\phi, \theta) \simeq \frac{1}{s} \sum_{i=1}^{s} \log p_{\theta}(x|z_{i}) - \log q_{\phi}(z_{i})
\end{equation}

By derivative with respect to $\theta$ we have:

\begin{equation}
    \nabla_{\theta} \mathcal{L}(\phi, \theta) \simeq \frac{1}{s} \sum_{i=1}^{s} \nabla_{\theta}  \log p_{\theta}(x|z_{i})
\end{equation}
because $q_{\phi}(z_{i})$ is independent of $\theta$. Since the expectation in equation \ref{eq:2.17} depends on $\phi$, it is not possible to calculate the gradient directly, so we use a reparameterization trick: instead of sampling $\{z_{i}\}_{i=1}^s$  from 
\begin{center}

$z \sim q_{\phi}(z) = \mathcal{N}(\mu_{\phi}(x), \sigma_{\phi}(x) ^ 2 \times I)$
    
\end{center}
we sample $\{\epsilon_{i}\}_{i=1}^s$ from a standard normal distribution
    $\epsilon \sim \mathcal{N}(0,I)$
and define a function $g_{x, \phi}(\epsilon)$ wich map $\epsilon$ to $z$:
\begin{equation}
    z = g_{x, \phi}(\epsilon) = \mu_{\phi}(x) + \sigma_{\phi}(x) \odot \epsilon
\end{equation}
Then by simply replacing parameter $g_{x, \phi}(\epsilon)$ instead of $z$ in equation \ref{eq:2.17} we have:

\begin{equation} \label{eq:2.21}
     \mathcal{L}(\phi, \theta) = \mathbb{E}_{\epsilon \sim \mathcal{N}(0,I)}[\log \frac{p(g_{x, \phi}(\epsilon))p_{\theta}(x|g_{x, \phi}(\epsilon))}{q_{\phi}(g_{x, \phi}(\epsilon))}]
\end{equation}
Now it is possible to compute $\nabla_{\phi}\mathcal{L}(\phi, \theta)$ as the same way we did for $\theta$.

Here, we apply the SGA to calculate $\phi$ and $\theta$ according the following flowchart:

% \begin{center}
% \includegraphics[scale=0.08]{Figures/theta_and_phi_opt.jpg} 
% \end{center}

which $M, \alpha$ are number of samples in every minibatch and learning rate, respectively. 

we can summarize the VAE operation as follow:

input $X$ $\longmapsto$ encode to statistics vectors $\longmapsto$ sample a latent vector $Z$ $\longmapsto$ decode $\longmapsto$ output $\hat{X}$
\textcolor{red}{graph if need!}

\subsubsection{The loss function}
In variational Auto-encoders loss function has two terms: one is reconstruction loss and another is $\mathcal{KL}$ Divergence.

$\mathcal{KL}$ divergence measures difference between distributions such as equation 2.2: \textcolor{red}{There is a graph here that I will draw}
\begin{equation}
D_{\mathcal{KL}} = \int p(x) \log \frac{p(x)}{q(x)}dx
\end{equation}
